# Supplementary material for: A Hybrid Transformer-Mamba Network for Single Image Deraining
Source: arXiv:2409.00410 source file (2024-08-31)
Supplement: Supplementary file 1 [file rain200h_supple.tex]

\begin{figure*}
  \centering
  \begin{minipage}{0.120\linewidth}
    \centering
  \begin{subfigure}{1\linewidth}
    \includegraphics[width=1\linewidth]{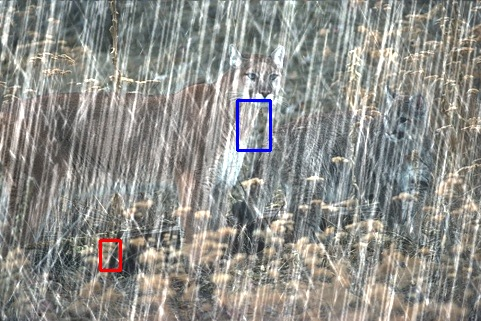}
  \end{subfigure}
    \hfill
     \begin{subfigure}{0.488\linewidth}
    \includegraphics[width=1\linewidth]{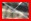}
    \end{subfigure}
    \hspace{-1.3mm}
     \begin{subfigure}{0.488\linewidth}
    \includegraphics[width=1\linewidth]{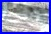}
    \end{subfigure}
    \hfill
  \begin{subfigure}{1\linewidth}
    \includegraphics[width=1\linewidth]{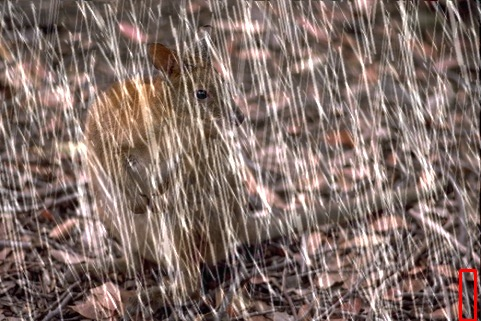}
  \end{subfigure}
    \hfill
     \begin{subfigure}{1\linewidth}
    \includegraphics[width=1\linewidth]{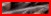}
    \end{subfigure}
    \subcaption[]{Input}
    \end{minipage}
  % \hfill
  % \begin{minipage}{0.120\linewidth}
  %   \centering
  % \begin{subfigure}{1\linewidth}
  %   \includegraphics[width=1\linewidth]{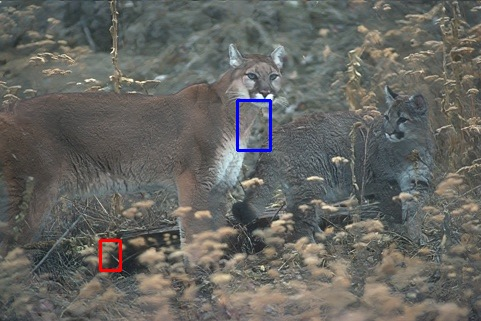}
  % \end{subfigure}
  %   \hfill
  %    \begin{subfigure}{1\linewidth}
  %   \includegraphics[width=1\linewidth]{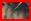}
  %   \end{subfigure}
  %   \hfill
  % \begin{subfigure}{1\linewidth}
  %   \includegraphics[width=1\linewidth]{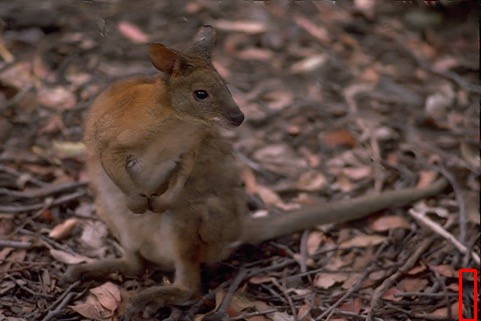}
  % \end{subfigure}
  %   \hfill
  %    \begin{subfigure}{1\linewidth}
  %   \includegraphics[width=1\linewidth]{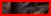}
  %   \end{subfigure}
  %   \subcaption[]{DualGCN}
  %   \end{minipage}
  \hfill
  \begin{minipage}{0.120\linewidth}
    \centering
  \begin{subfigure}{1\linewidth}
    \includegraphics[width=1\linewidth]{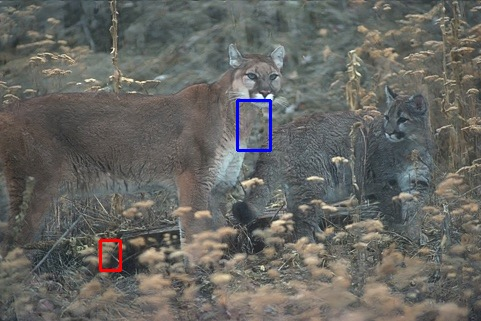}
  \end{subfigure}
    \hfill
     \begin{subfigure}{0.488\linewidth}
    \includegraphics[width=1\linewidth]{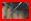}
    \end{subfigure}
    \hspace{-1.3mm}
     \begin{subfigure}{0.488\linewidth}
    \includegraphics[width=1\linewidth]{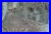}
    \end{subfigure}
    \hfill
  \begin{subfigure}{1\linewidth}
    \includegraphics[width=1\linewidth]{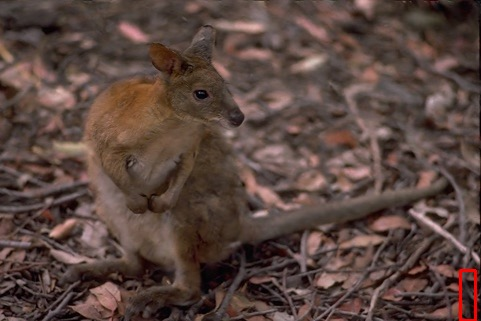}
  \end{subfigure}
    \hfill
     \begin{subfigure}{1\linewidth}
    \includegraphics[width=1\linewidth]{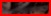}
    \end{subfigure}
    \subcaption[]{SPDNet}
    \end{minipage}
  \hfill
  \begin{minipage}{0.120\linewidth}
    \centering
  \begin{subfigure}{1\linewidth}
    \includegraphics[width=1\linewidth]{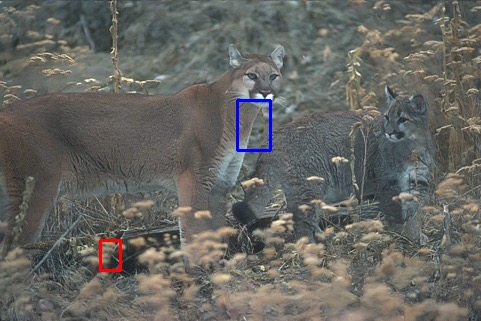}
  \end{subfigure}
    \hfill
     \begin{subfigure}{0.488\linewidth}
    \includegraphics[width=1\linewidth]{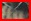}
    \end{subfigure}
    \hspace{-1.3mm}
     \begin{subfigure}{0.488\linewidth}
    \includegraphics[width=1\linewidth]{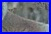}
    \end{subfigure}
    \hfill
  \begin{subfigure}{1\linewidth}
    \includegraphics[width=1\linewidth]{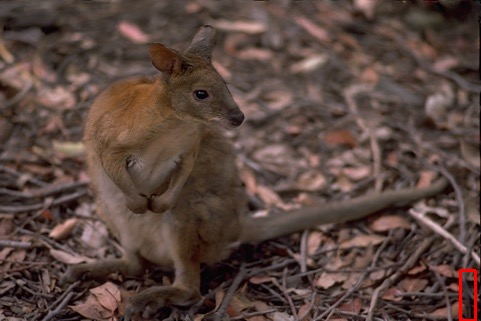}
  \end{subfigure}
    \hfill
     \begin{subfigure}{1\linewidth}
    \includegraphics[width=1\linewidth]{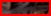}
    \end{subfigure}
    \subcaption[]{Restormer}
    \end{minipage}
  \hfill
  \begin{minipage}{0.120\linewidth}
    \centering
  \begin{subfigure}{1\linewidth}
    \includegraphics[width=1\linewidth]{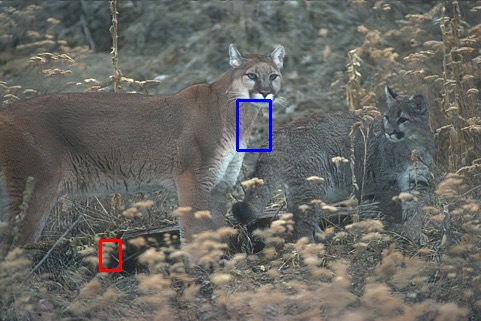}
  \end{subfigure}
    \hfill
     \begin{subfigure}{0.488\linewidth}
    \includegraphics[width=1\linewidth]{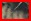}
    \end{subfigure}
    \hspace{-1.3mm}
     \begin{subfigure}{0.488\linewidth}
    \includegraphics[width=1\linewidth]{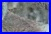}
    \end{subfigure}
    \hfill
  \begin{subfigure}{1\linewidth}
    \includegraphics[width=1\linewidth]{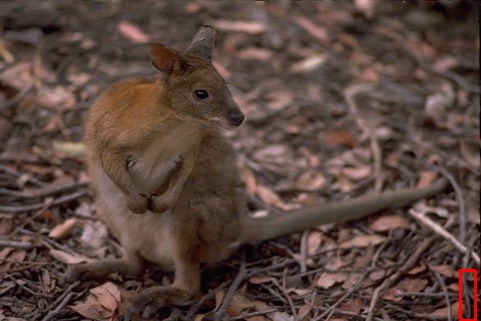}
  \end{subfigure}
    \hfill
     \begin{subfigure}{1\linewidth}
    \includegraphics[width=1\linewidth]{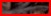}
    \end{subfigure}
    \subcaption[]{IDT}
    \end{minipage}
  \hfill
  \begin{minipage}{0.120\linewidth}
    \centering
  \begin{subfigure}{1\linewidth}
    \includegraphics[width=1\linewidth]{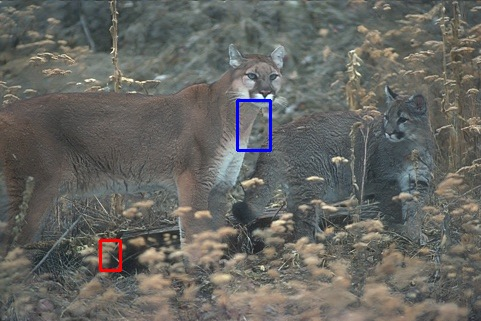}
  \end{subfigure}
    \hfill
     \begin{subfigure}{0.488\linewidth}
    \includegraphics[width=1\linewidth]{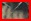}
    \end{subfigure}
    \hspace{-1.3mm}
     \begin{subfigure}{0.488\linewidth}
    \includegraphics[width=1\linewidth]{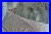}
    \end{subfigure}
    \hfill
  \begin{subfigure}{1\linewidth}
    \includegraphics[width=1\linewidth]{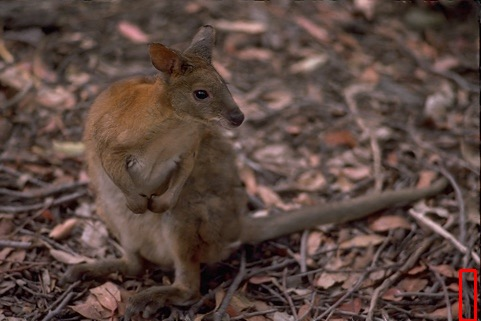}
  \end{subfigure}
    \hfill
     \begin{subfigure}{1\linewidth}
    \includegraphics[width=1\linewidth]{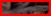}
    \end{subfigure}
    \subcaption[]{DRSformer}
    \end{minipage}
  \hfill
  \begin{minipage}{0.120\linewidth}
    \centering
  \begin{subfigure}{1\linewidth}
    \includegraphics[width=1\linewidth]{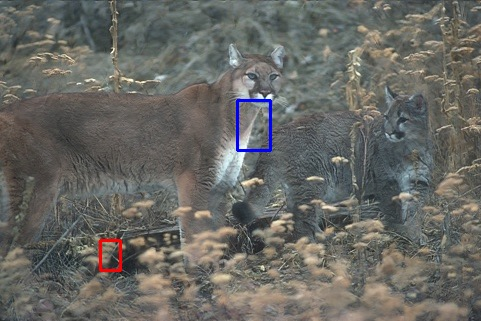}
  \end{subfigure}
    \hfill
     \begin{subfigure}{0.488\linewidth}
    \includegraphics[width=1\linewidth]{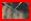}
    \end{subfigure}
    \hspace{-1.3mm}
     \begin{subfigure}{0.488\linewidth}
    \includegraphics[width=1\linewidth]{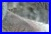}
    \end{subfigure}
    \hfill
  \begin{subfigure}{1\linewidth}
    \includegraphics[width=1\linewidth]{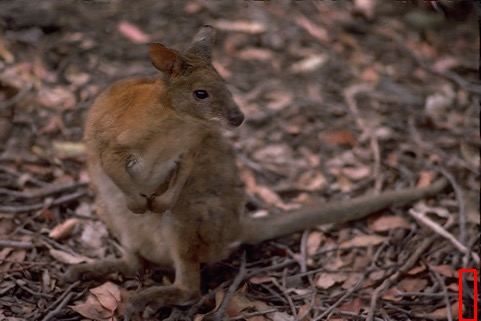}
  \end{subfigure}
    \hfill
     \begin{subfigure}{1\linewidth}
    \includegraphics[width=1\linewidth]{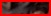}
    \end{subfigure}
    \subcaption[]{\scriptsize UDR-S$^2$Former}
    \end{minipage}
  \hfill
  \begin{minipage}{0.120\linewidth}
    \centering
  \begin{subfigure}{1\linewidth}
    \includegraphics[width=1\linewidth]{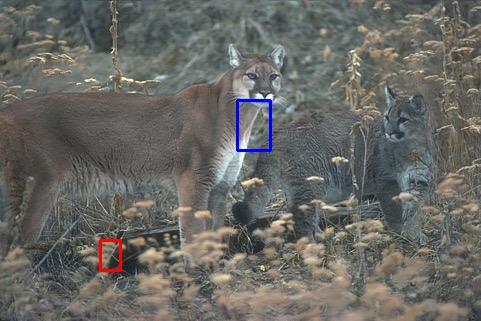}
  \end{subfigure}
    \hfill
     \begin{subfigure}{0.488\linewidth}
    \includegraphics[width=1\linewidth]{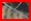}
    \end{subfigure}
    \hspace{-1.3mm}
     \begin{subfigure}{0.488\linewidth}
    \includegraphics[width=1\linewidth]{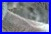}
    \end{subfigure}
    \hfill
  \begin{subfigure}{1\linewidth}
    \includegraphics[width=1\linewidth]{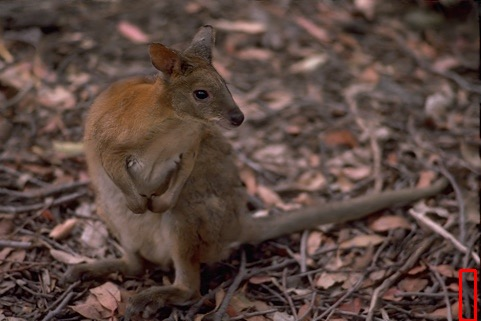}
  \end{subfigure}
    \hfill
     \begin{subfigure}{1\linewidth}
    \includegraphics[width=1\linewidth]{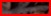}
    \end{subfigure}
    \subcaption[]{Ours}
    \end{minipage}
  \hfill
  \begin{minipage}{0.120\linewidth}
    \centering
  \begin{subfigure}{1\linewidth}
    \includegraphics[width=1\linewidth]{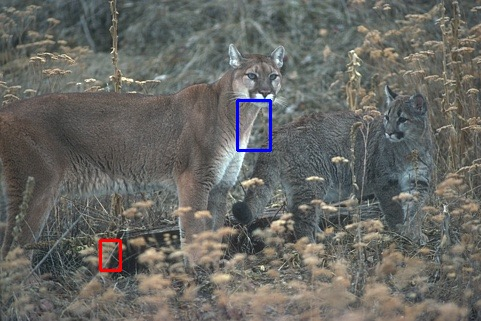}
  \end{subfigure}
    \hfill
     \begin{subfigure}{0.488\linewidth}
    \includegraphics[width=1\linewidth]{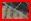}
    \end{subfigure}
    \hspace{-1.3mm}
     \begin{subfigure}{0.488\linewidth}
    \includegraphics[width=1\linewidth]{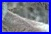}
    \end{subfigure}
    \hfill
  \begin{subfigure}{1\linewidth}
    \includegraphics[width=1\linewidth]{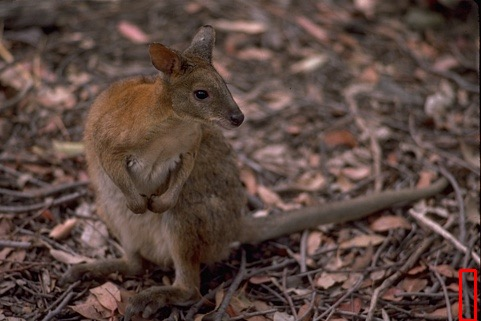}
  \end{subfigure}
    \hfill
     \begin{subfigure}{1\linewidth}
    \includegraphics[width=1\linewidth]{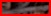}
    \end{subfigure}
    \subcaption[]{Ground-truth}
    \end{minipage}
    \vspace{-3mm}
  \caption{Visual comparisons of deraining on Rain200H~\cite{yang2017deep}. Please zoom in for a better view.}
  \label{fig:rain200H_supple}
  \vspace{-3mm}
\end{figure*}
