# Supplementary material for: A Hybrid Transformer-Mamba Network for Single Image Deraining
Source: arXiv:2409.00410 source file (2024-08-31)
Supplement: Supplementary file 5 [file real-supple-3.tex]

\begin{figure*}
  \centering
  \begin{minipage}{0.495\linewidth}
    \centering
  \begin{subfigure}{1\linewidth}
    \includegraphics[width=1\linewidth]{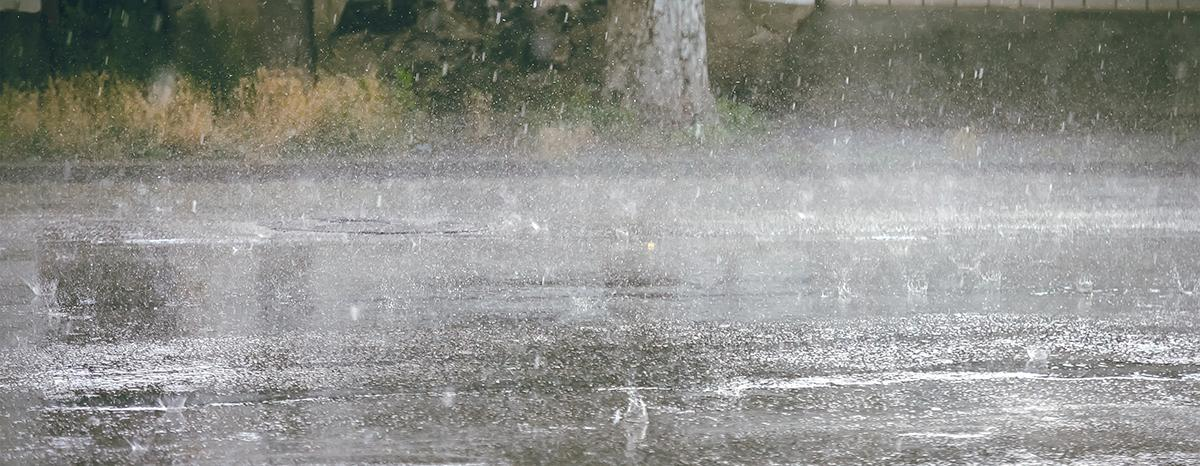}
  \end{subfigure}
    \subcaption[]{Input}
    \end{minipage}
  \hfill
  \begin{minipage}{0.495\linewidth}
    \centering
  \begin{subfigure}{1\linewidth}
    \includegraphics[width=1\linewidth]{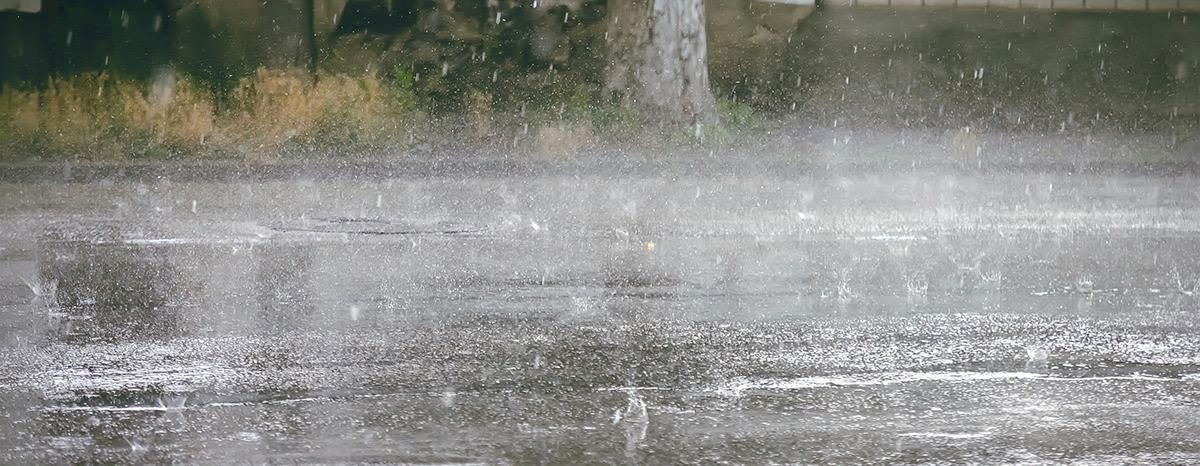}
  \end{subfigure}
    \subcaption[]{DualGCN~\cite{Fu2021RainSR}}
    \end{minipage}
  \hfill
  \begin{minipage}{0.495\linewidth}
    \centering
  \begin{subfigure}{1\linewidth}
    \includegraphics[width=1\linewidth]{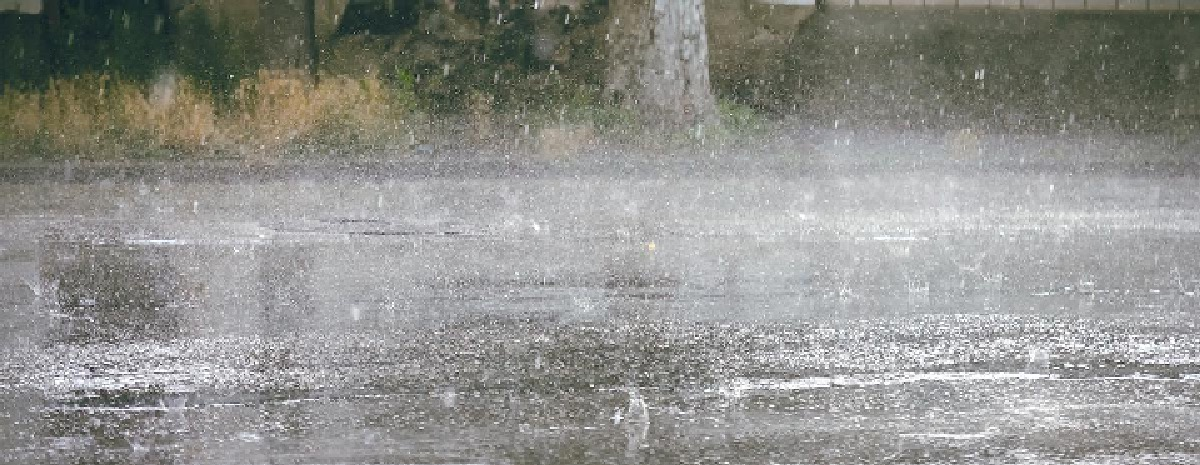}
  \end{subfigure}
    \subcaption[]{SPDNet~\cite{yi2021Structure}}
    \end{minipage}
  \hfill
  \begin{minipage}{0.495\linewidth}
    \centering
  \begin{subfigure}{1\linewidth}
    \includegraphics[width=1\linewidth]{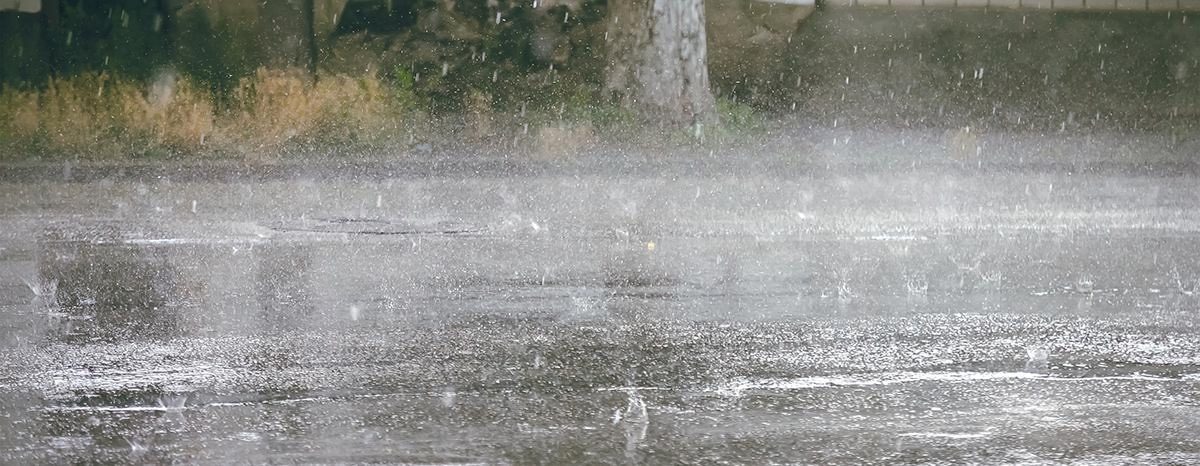}
  \end{subfigure}
    \subcaption[]{Restormer~\cite{zamir2022restormer}}
    \end{minipage}
  \hfill
  \begin{minipage}{0.495\linewidth}
    \centering
  \begin{subfigure}{1\linewidth}
    \includegraphics[width=1\linewidth]{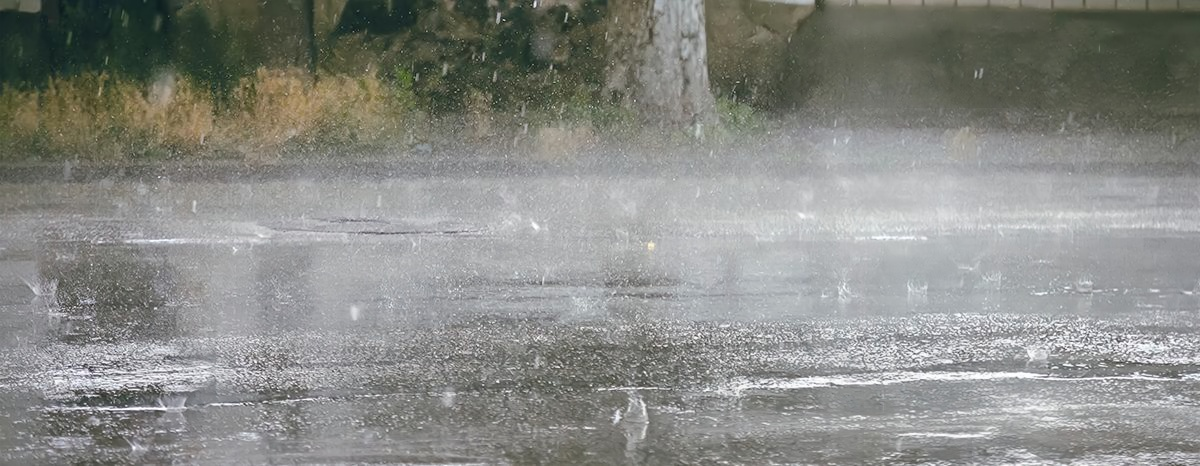}
  \end{subfigure}
    \subcaption[]{IDT~\cite{xiao2022image}}
    \end{minipage}
  \hfill
  \begin{minipage}{0.495\linewidth}
    \centering
  \begin{subfigure}{1\linewidth}
    \includegraphics[width=1\linewidth]{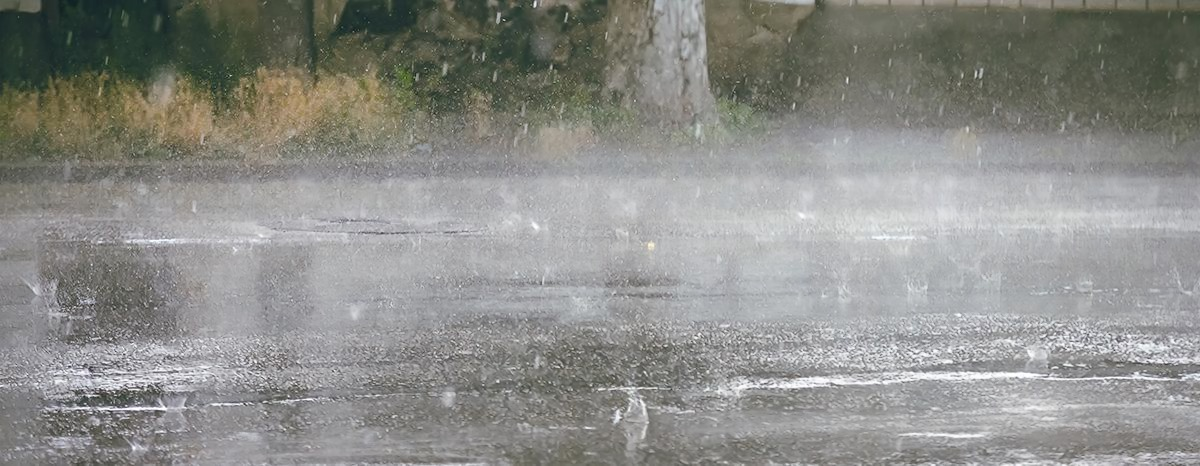}
  \end{subfigure}
    \subcaption[]{DRSformer~\cite{chen2023learning}}
    \end{minipage}
  \hfill
  \begin{minipage}{0.495\linewidth}
    \centering
  \begin{subfigure}{1\linewidth}
    \includegraphics[width=1\linewidth]{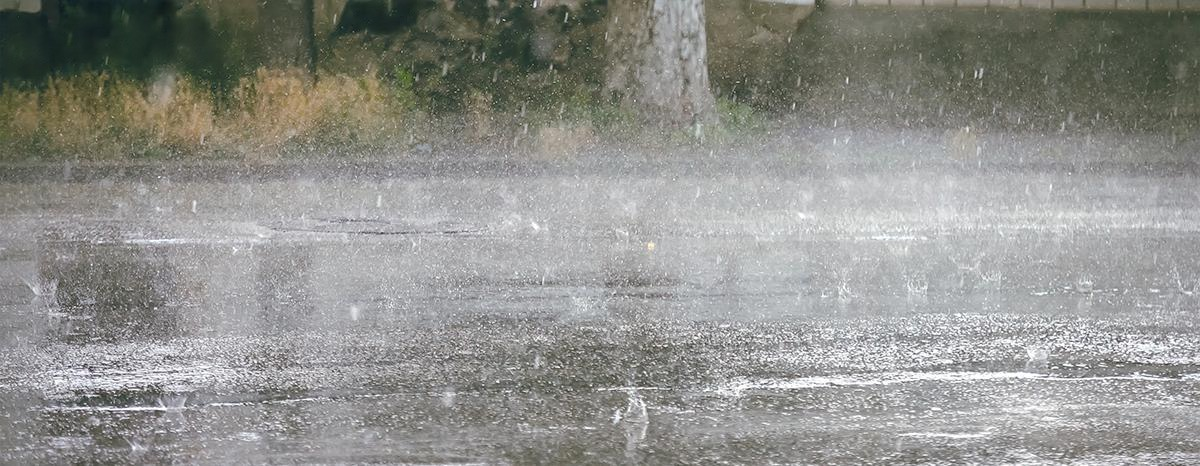}
  \end{subfigure}
    \subcaption[]{UDR-S$^2$Former~\cite{chen2023sparse}}
    \end{minipage}
  \hfill
  \begin{minipage}{0.495\linewidth}
    \centering
  \begin{subfigure}{1\linewidth}
    \includegraphics[width=1\linewidth]{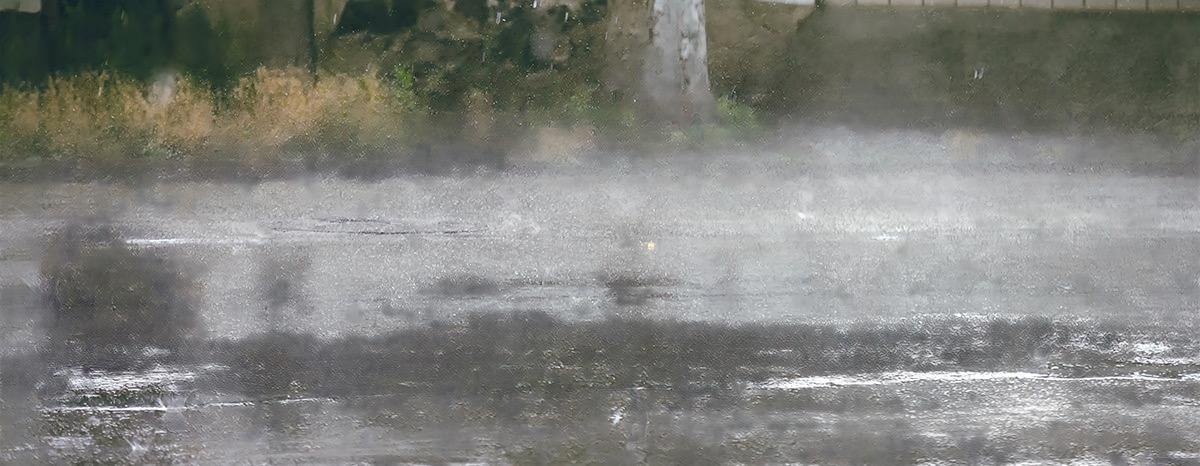}
  \end{subfigure}
    \subcaption[]{Ours}
    \end{minipage}
  \caption{A visual comparison of deraining on Internet-Data~\cite{wang2019spatial}.}
  \label{fig:real-supple-3}
\end{figure*}
